# Supplementary material for: Deep Learning-Based Out-of-distribution Source Code Data Identification: How Far Have We Gone?
Source: arXiv:2404.05964 source file (2024-04-15)
Supplement: Supplementary file 1 [file appendix.tex]

\section{Appendix}\label{sec:appendix}

\subsection{Data processing and embedding\label{sec:datape}}

We preprocessed the datasets before injecting them into deep neural networks. In particular, we standardized the source code by (i) removing comments, blank lines, and non-ASCII characters, and (ii) mapping user-defined variables to symbolic variable names (e.g., \emph{var1} and \emph{var2}) and user-defined
functions to symbolic function names (e.g., \emph{func1} and \emph{func2}) using Treesitter \cite{Treesitter}.  We also replaced strings with a generic \emph{"str"} token.

We then embedded source code statements into vectors. For instance, consider the following statement (C/C++ programming language) \emph{"for(var1=0;var1<10;var1++)"}, we use the byte pair encoding (BPE) algorithm \cite{sennrich2016neural} (i.e., commonly used in large language models, e.g., CodeBERT \cite{CodeBERT2020} for tokenization) to tokenize this statement into a sequence of tokens, and then we used a 150-dimensional token Embedding layer followed by a Dropout layer with a dropped fixed probability $p=0.2$ and (a 1D convolutional layer with the filter size $150$ and kernel size $3$, and a 1D max pooling layer) or (a 1D max pooling layer) to encode each statement in a function $F$. Finally, a mini-batch of functions in which each function consisting of $L$ encoded statements was fed to the deep learning-based models. Note that the Embedding and convolutional layers are learnable during the training process.

It is worth noting that the length ($L$) of each function is padded or truncated to $100$ source code statements. We chose these values based on the fact that for the used dataset, over 95\% of the source code functions, have the
number of code statements less than or equal to $100$. Furthermore, almost all important information relevant to the vulnerability of each source
code function lies in the first $100$ code statements.

\subsection{Model's configurations}\label{sec:modelc}

For the main baselines of our \textbf{\ourapp~}method including \textbf{Standard DNN} \cite{Hendrycks2017dnn}, \textbf{Outlier Exposure} \cite{Hendrycks18}, and \textbf{SSD} \cite{Sehwag21}. These methods are popular and state-of-the-art approaches for out-of-distribution detection applied in the computer vision domain. To make them applicable for out-of-distribution source code vulnerability detection, we keep the principle of these methods and use the same data embedding process for handling the sequential source code data as used in our method. For the popular and state-of-the-art baselines (i.e., \textbf{VulDeePecker} \cite{VulDeePecker2018}, \textbf{CodeBERT} \cite{CodeBERT2020}, and \textbf{ReGVD} \cite{ReGVD2022}) in the software vulnerability detection problem, we use the architecture proposed in the corresponding original papers.

To our \ourapp~ method, for the $g\left(\cdot;\alpha\right)$
and $f\left(\cdot;\beta\right)$ networks, we used deep feed-forward neural networks having three and two hidden layers with the size of each hidden layer in $\left\{100,300\right\} $. The dense hidden layers are followed by a ReLU function as nonlinearity and Dropout \cite{srivastava14a} with a retained fixed probability $p=0.8$ as regularization. The last dense layer of the $g\left(\cdot;\alpha\right)$ network for learning a discrete distribution is followed by a sigmoid function while the last dense layer of the $f\left(\cdot;\beta\right)$ network is followed by a softmax function for predicting. The number of chosen clusters guiding the computation of the innovative cluster-contrastive learning mentioned is from $2$ to $5$ in the case of the distribution data consisting of one vulnerability type. When the in-distribution data consists of more than one vulnerability type, the number of vulnerability patterns used in cluster-contrastive learning also needs to be increased. In the cases of two or more two vulnerability types (i.e., three), we vary and tune the number of clusters in the range of $2$ to $15$.
The trade-off hyper-parameter $\lambda$ representing the weight of the innovative cluster-contrastive learning is in $\{10^{-2},10^{-1},10^{0}\}$ while the scalar temperature $\tau$ is in $\{0.5, 1.0\}$. The temperature $\nu$ for the Gumbel softmax distribution is also set in $\{0.5, 1.0\}$.

For our \ourapp~ method and baselines, we employed
the Adam optimizer \cite{KingmaB14} with an initial learning rate
equal to $10^{-3}$, while the mini-batch size is set to $128$. For the training process, we split the data of each in-distribution data set into two random partitions. The first partition contains 80\% for training, the second partition contains 20\% for validation. For each in-distribution data set, we used $10$ epochs for the training process. We additionally applied gradient clipping regularization to prevent over-fitting. For each method, we ran the corresponding model several times and reported the averaged FPR (at TPR 95\%), AUROC, and AUPR measures. We ran our experiments in Python
using Tensorflow \cite{abadi2016tensorflow} for the used methods
on a 13th Gen Intel(R) Core(TM) i9-13900KF having 24 CPU Cores at 3.00 GHz with 32GB RAM, integrated Gigabyte RTX 4090 Gaming OC 24GB. Some baseline methods (i.e., \textbf{CodeBERT} \cite{CodeBERT2020} and \textbf{ReGVD} \cite{ReGVD2022}) were written using Pytorch \cite{pytorch2019}. For these baselines, we followed the source code samples published by the authors.

\subsection{Discussion of Threats to Validity }\label{sec:discussion}

\paragraph{Construct Validity}
Key construct validity threats are if our assessments of the proposed method and baselines demonstrate their capability for out-of-distribution source code vulnerability detection. In the cyber security domain, by doing out-of-distribution vulnerability detection, we help security analysts and software engineers detect potential unknown vulnerability types coming in order to harden the security computer systems. To evaluate the performance of our method and baselines, we use three main common measures used in out-of-distribution detection including \textbf{FPR} (at TPR 95\%), \textbf{AUROC}, and \textbf{AUPR}.

\paragraph{Internal Validity}
Key internal validity threats are relevant to the choice of hyper-parameter settings (i.e., optimizer, learning rate, number of layers in deep neural networks, etc.). It is worth noting that finding a set of optimal hyperparameter settings of deep neural networks is expensive due to a large number of trainable parameters. To train our method, we only use the common or default values for the hyper-parameters such as using Adam optimizer, the learning rate equals $10^{-3}$, while the scalar temperature $\tau$ used in the cluster-contrastive learning and the temperature $\nu$ for the Gumbel softmax distribution are set in $\{0.5, 1.0\}$. For the number of clusters used in cluster-contrastive learning aiming to improve the data representation learning process, we use it as a hyperparameter. In our paper, we detail the hyperparameter settings (i.e., the value-tuned ranges of the hyperparameters) in the released reproducible source code to support future replication studies.

\paragraph{External Validity}
Key external validity threats include whether our proposed \ourapp~ method will generalize to other source code vulnerability types and whether they will work on other types of vulnerability datasets. We mitigated this problem by conducting our experiments on the top five popular (CWE) vulnerability types as mentioned in \cite{Bigdata2020} including CWE-119 (Improper Restriction of Operations within the Bounds of a Memory Buffer), CWE-20 (Improper Input Validation), CWE-125 (Out-of-bounds Read), CWE-200 (Exposure of Sensitive Information to an Unauthorized Actor), and CWE-264 (Permissions, Privileges, and Access Controls).

\subsection{Additional experiments}\label{sec:additionale}
Here we present some additional experiments of our \ourapp~ method and baselines on other further cases of the in-distribution and out-of-distribution source code vulnerability data. The experimental results in Table \ref{tab:my_label_app} again show the effectiveness and superiority of our proposed \ourapp~ method compared to the baselines for out-of-distribution software vulnerability detection by a wide margin. Notably, in these additional cases, our method obtains around (10\% to 95\%), (4\% to 53\%), and (3.6\% to 89\%) higher performances on the FPR (at TPR 95\%), AUROC, and AUPR measures, respectively, compared to the baselines.

\begin{table}[ht]
\centering{}
\resizebox{0.93\columnwidth}{!}{
\begin{tabular}{ccrrr}
\hline 
%\textbf{ID and OOD Datasets} & \textbf{Methods} & \textbf{FPR} $\downarrow$ & \textbf{AUROC} $\uparrow$ & \textbf{AUPR} $\uparrow$
\textbf{ID and OOD} & \textbf{Methods} & \textbf{FPR} $\downarrow$& \textbf{AUROC} $\uparrow$& \textbf{AUPR} $\uparrow$
\tabularnewline
\hline 
 
\multirow{7}{*}{CWE20 vs. CWE264}
&  Standard DNN & 89.58\%	& 76.48\%	& 17.40\%
\tabularnewline
%\cline{2-5} \cline{3-5} \cline{4-5} \cline{5-5} 
&  Outlier Exposure & 91.93\% &  78.86\% &  18.00\%  
\tabularnewline
%\cline{2-5} \cline{3-5} \cline{4-5} \cline{5-5} 
&  SSD & 88.28\%	& 86.27\%	& 26.44\%
\tabularnewline
%\cline{2-5} \cline{3-5} \cline{4-5} \cline{5-5} 
&  VulDeePecker & \underline{72.14\%}	& \underline{92.33\%}	& \underline{37.41\%}
\tabularnewline
%\cline{2-5} \cline{3-5} \cline{4-5} \cline{5-5} 
&  CodeBERT  & 90.31\%	& 48.86\%	& 13.21\%
\tabularnewline
%\cline{2-5} \cline{3-5} \cline{4-5} \cline{5-5} 
&  ReGVD & 91.13\%	& 63.96\%	& 15.80\%
\tabularnewline
\cline{2-5} \cline{3-5} \cline{4-5} \cline{5-5} 
&  \multirow{2}{*}{\ourapp~ (Ours)}  & \textbf{0.00\%} & \textbf{99.63\%} & \textbf{92.77\%}
\tabularnewline
%\cline{3-5} \cline{4-5} \cline{5-5} 
 &  & \textcolor{blue}{($\downarrow$ 72.14\%)} & \textcolor{blue}{($\uparrow$ 7.3\%)} & \textcolor{blue}{($\uparrow$ 55.36\%)}\tabularnewline
\hline

\multirow{7}{*}{CWE200 vs. CWE119}
&  Standard DNN & 88.02\%	& 77.84\%	& 71.74\%
\tabularnewline
%\cline{2-5} \cline{3-5} \cline{4-5} \cline{5-5} 
&  Outlier Exposure &  84.79\%	& 82.74\%	& 76.94\%
\tabularnewline
%\cline{2-5} \cline{3-5} \cline{4-5} \cline{5-5} 
&  SSD & 88.23\%	& 80.88\%	& 74.28\%
\tabularnewline
%\cline{2-5} \cline{3-5} \cline{4-5} \cline{5-5} 
&  VulDeePecker & \underline{24.58\%}	& \underline{94.60\%}	& \underline{95.49\%}
\tabularnewline
%\cline{2-5} \cline{3-5} \cline{4-5} \cline{5-5} 
&  CodeBERT  & 58.16\%	& 72.91\% & 80.98\%
\tabularnewline
%\cline{2-5} \cline{3-5} \cline{4-5} \cline{5-5} 
&  ReGVD  & 95.58\%	& 55.13\%	& 56.73\%
\tabularnewline
\cline{2-5} \cline{3-5} \cline{4-5} \cline{5-5} 
%&  \ourapp~ (Ours)  & \textbf{0.00\%} & \textbf{99.32\%} & \textbf{99.05\%}
%\tabularnewline

& \multirow{2}{*}{LEO (Ours)} & \textbf{0.00\%} & \textbf{99.32\%} & \textbf{99.05\%}\tabularnewline
%\cline{3-5} \cline{4-5} \cline{5-5} 
 &  & \textcolor{blue}{($\downarrow$ 24.58\%)} & \textcolor{blue}{($\uparrow$ 4.72\%)} & \textcolor{blue}{($\uparrow$ 3.56\%)}\tabularnewline

 \hline
\multirow{7}{*}{CWE200 vs. CWE264}
&  Standard DNN & 93.49\%	& 67.11\%	& 25.40\%
\tabularnewline
%\cline{2-5} \cline{3-5} \cline{4-5} \cline{5-5} 
&  Outlier Exposure &  91.67\%	& 75.52\%	& 31.59\%
\tabularnewline
%\cline{2-5} \cline{3-5} \cline{4-5} \cline{5-5} 
&  SSD & 87.24\%	& \underline{80.50\%}	& 37.54\%
\tabularnewline
%\cline{2-5} \cline{3-5} \cline{4-5} \cline{5-5} 
&  VulDeePecker & 65.36\%	& 74.24\%	& 53.21\%
\tabularnewline
%\cline{2-5} \cline{3-5} \cline{4-5} \cline{5-5} 
&  CodeBERT  & \underline{60.00\%}	& 70.74\%	& \underline{57.74\%}
\tabularnewline
%\cline{2-5} \cline{3-5} \cline{4-5} \cline{5-5} 
&  ReGVD  & 95.46\%	& 54.03\%	& 23.88\%
\tabularnewline
\cline{2-5} \cline{3-5} \cline{4-5} \cline{5-5} 
&  \multirow{2}{*}{\ourapp~ (Ours)}  & \textbf{0.00\%} & \textbf{99.91\%} & \textbf{99.26\%}
\tabularnewline
%\cline{3-5} \cline{4-5} \cline{5-5} 
 &  & \textcolor{blue}{($\downarrow$ 60.00\%)} & \textcolor{blue}{($\uparrow$ 19.41\%)} & \textcolor{blue}{($\uparrow$ 41.52\%)}\tabularnewline
\hline

%\hline
\multirow{7}{*}{CWE264 vs. CWE20}
&  Standard DNN & 91.80\%	& 62.03\%	& 38.20\%
\tabularnewline
%\cline{2-5} \cline{3-5} \cline{4-5} \cline{5-5} 
&  Outlier Exposure &  83.50\% &  72.09\% & 48.95\%
\tabularnewline
%\cline{2-5} \cline{3-5} \cline{4-5} \cline{5-5} 
&  SSD & 85.84\%	& 82.97\%	& 59.62\%
\tabularnewline
%\cline{2-5} \cline{3-5} \cline{4-5} \cline{5-5} 
&  VulDeePecker & 52.34\%	& 90.88\%	& 74.79\%
\tabularnewline
%\cline{2-5} \cline{3-5} \cline{4-5} \cline{5-5} 
&  CodeBERT  & \underline{10.06\%}	& \underline{95.57\%}	& \underline{95.31\%}
\tabularnewline
%\cline{2-5} \cline{3-5} \cline{4-5} \cline{5-5} 
&  ReGVD  & 90.12\%	& 68.36\%	& 43.88\%
\tabularnewline
\cline{2-5} \cline{3-5} \cline{4-5} \cline{5-5} 
&  \multirow{2}{*}{\ourapp~ (Ours)}  & \textbf{0.00\%} & \textbf{99.82\%} & \textbf{99.32\%}
\tabularnewline
%\cline{3-5} \cline{4-5} \cline{5-5} 
 &  & \textcolor{blue}{($\downarrow$ 10.06\%)} & \textcolor{blue}{($\uparrow$ 4.25\%)} & \textcolor{blue}{($\uparrow$ 4.01\%)}\tabularnewline
\hline
%\hline

 \multirow{7}{*}
 &  Standard DNN & 80.08\%	& \underline{90.47\%}	& 18.27\%
 \tabularnewline
%\cline{2-5} \cline{3-5} \cline{4-5} \cline{5-5} 
 &  Outlier Exposure &  86.52\%	& 85.44\%	& 12.84\%
 \tabularnewline
%\cline{2-5} \cline{3-5} \cline{4-5} \cline{5-5} 
{CWE119-20-264}
 &  SSD & 94.34\%	& 79.86\%	& 9.32\%
 \tabularnewline
%\cline{2-5} \cline{3-5} \cline{4-5} \cline{5-5} 
vs. {CWE125}
 &  VulDeePecker & \underline{54.69\%}	& 88.76\%	& \underline{33.41\%}
 \tabularnewline
%\cline{2-5} \cline{3-5} \cline{4-5} \cline{5-5} 
 &  CodeBERT & 90.06\%	& 47.02\%	& 19.17\%
 \tabularnewline
%\cline{2-5} \cline{3-5} \cline{4-5} \cline{5-5} 
 &  ReGVD  & 87.02\%	& 69.85\%	& 8.35\%
 \tabularnewline
\cline{2-5} \cline{3-5} \cline{4-5} \cline{5-5} 
 %&  \ourapp~ (Ours)  & \textbf{0.26\%} & \textbf{99.75\%} & \textbf{92.44\%}
 %\tabularnewline
 & \multirow{2}{*}{\ourapp~ (Ours)} & \textbf{0.00\%} & \textbf{99.93\%} & \textbf{97.06\%}\tabularnewline
%\cline{3-5} \cline{4-5} \cline{5-5} 
 &  & \textcolor{blue}{($\downarrow$ 54.69\%)} & \textcolor{blue}{($\uparrow$ 9.46\%)} & \textcolor{blue}{($\uparrow$ 63.65\%)}\tabularnewline
 \hline
\end{tabular}}
\vspace{-1mm}
\caption{The results of our \ourapp~ method and baselines for the FPR (at TPR 95\%), AUROC, and AUPR measures on the vulnerable source code samples of each out-of-distribution data with the corresponding used in-distribution data. (The best results are in \textbf{bold} while the second highest results are in \underline{underline}. The numbers highlighted in blue color are the improvements of our method \ourapp~ over the second-best values from the baselines.)}\label{tab:my_label_app}
\vspace{-3mm}
\end{table}

\subsection{Related backgrounds}

In this section, we briefly present the main related backgrounds used in our proposed \ourapp~ and the baseline methods.

\subsubsection{\textbf{Recurrent neural networks}}

Recurrent neural networks (RNNs) \cite{Rumelhart-RNN86}, a class of deep neural networks (DNNs), are specialized for sequential data (e.g., time series, sentences, documents, or audio samples). RNNs are extremely useful for natural language processing (NLP) systems \cite{ChoMBB14,sutskever2014sequence}
such as automatic translation, speech-to-text, and sentiment analysis. Leveraging the idea of sharing parameters across different parts of a model, an RNN can extend and apply to data of different forms and generalize across them. An RNN is similar to a DNN, except it has backward connections.
A visualization of an RNN's architecture is depicted in Figure \ref{fig:architecture-of-rnn}
(the left-hand figure). At each time step $t$, the state of a recurrent
neuron (i.e., the hidden state denoted by $\bh_{t}$) will receive the input vector $\bx_{t}$ as well as the state vector from the previous step $t-1$ (i.e., $\bh_{t-1}$) to obtain the state vector $\bh_{t}$.

In particular, we have:
\[
\bh_{t}=f(\bh_{t-1},\bx_{t})
\]

We can unroll the RNN network through time to gain a new visualization as depicted in Figure \ref{fig:architecture-of-rnn} (the right-hand figure). Each recurrent neuron has two relevant input weights. One is for the input vector $\bx_{t}$, and the other is for the state vector $\bh_{t-1}$ of the previous time step $t-1$. At the time step $t$, if we denote the weight from the input vector $\bx_{t}$ to the state $\bh_{t}$ of the current recurrent neuron by $\bW_{xh}$ and the weight from the state $\bh_{t-1}$ of the previous recurrent neuron to the state $\bh_{t}$ of the current recurrent neuron by $\bW_{hh}$, the state $\bh_{t}$ of the current recurrent neuron is computed as follows:
\[
\bh_{t}=\phi(\bW_{xh}^{\top}\bx_{t}+\bW_{hh}^{\top}\bh_{t-1}+\bb)
\]

where $\bb$ is the bias vector and $\phi(.)$ is the activation function (e.g., the ReLU or Tanh functions).

At the time step $t$, if we denote $\bW_{hy}$ as the weight from the state $\bh_{t}$ of the current recurrent neuron to the corresponding output denoted by $\by_{t}$, the output $\by_{t}$ is computed as follows:

\[
\by_{t}=\phi(\bW_{hy}^{\top}\bh_{t}+\bc)
\]

where $\bc$ is the bias vector and $\phi(.)$ is the activation function (e.g., the softmax function).

\begin{figure}[h]
\begin{centering}
\includegraphics[width=0.96\columnwidth]{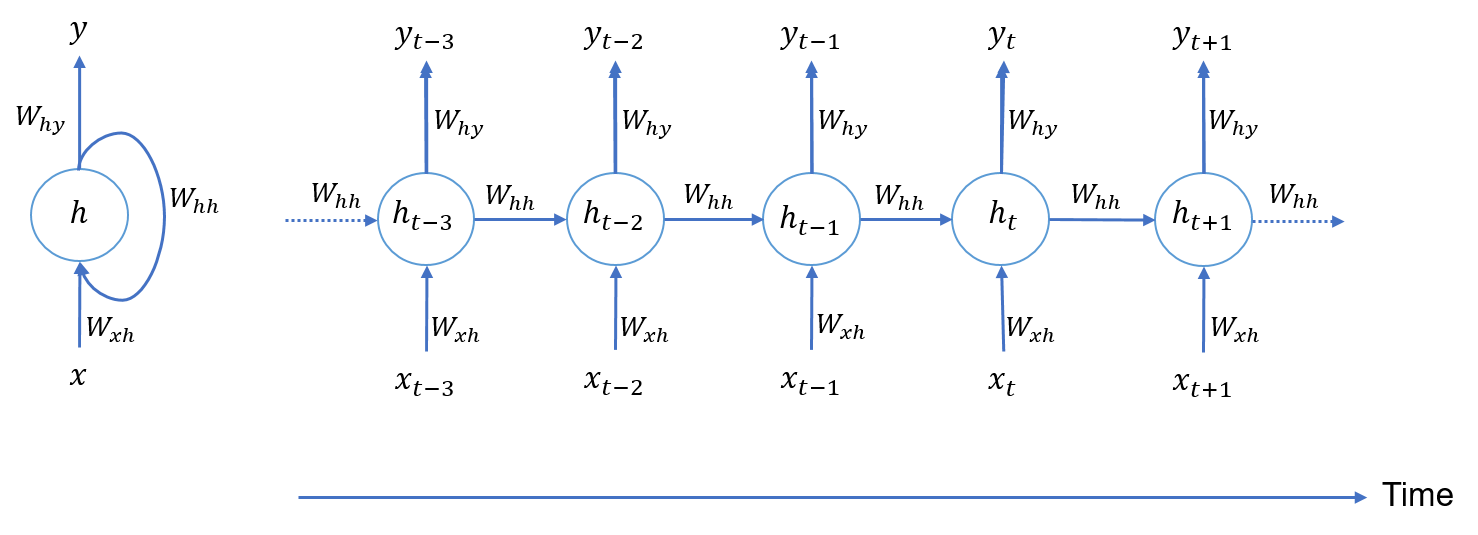}
\par\end{centering}
\caption{An Architecture of a recurrent neural network with the outputs $y$ plus the hidden states $h$ of recurrent neurons. \label{fig:architecture-of-rnn}}
\end{figure}

\subsubsection{\textbf{Long short-term memory networks}}

Long short-term memory (LSTM) networks are a type of RNNs capable of learning long-term dependencies, first proposed by Hochreiter and
Schmidhuber \cite{hochreiter1997long-short} and gradually improved over the years by other researches \cite{hasim-lstm-2014,zaremba-lstm-2014}. An LSTM network was introduced to address the exploding and vanishing gradients problems as well as the short-term memory problem (i.e., the lost information from some of the first elements from the corresponding input in the memory cell of a long RNN) in training RNNs.

The key idea of an LSTM network is about storing long-term memory. An LSTM network can learn to figure out what information from the inputs should be read and stored in the long-term state denoted by
$\bc_{t}$ as well as what information should be thrown out from $\bc_{t}$. A visualization of an LSTM network is shown in Figure \ref{fig:architecture-of-lstm}.
As depicted, there are four layers in an LSTM network including the main layer and three additional layers (i.e., gate controllers), namely, the forget gate, the input gate, and the output gate.
\begin{itemize}
\item The main layer at the time step $t$ aims to analyse the current input vector $\bx_{t}$ and the previous (short-term) state $\bh_{t-1}$ to gain the output $\bg_{t}$ (i.e., $\bh_{t}$ in a basic cell RNN). In an LSTM cell, the layer's output $\bg_{t}$ does not go straight out, but instead goes through a gate controller to decide what parts are stored in the long-term state (i.e., $\bc_{t}$).
\item Using the logistic activation function, the forget gate $\bff_{t}$ aims to learn which parts of the long-term state $\bc_{t}$ should be erased. The input gate $\bi_{t}$ aims to control which parts of $\bg_{t}$ should be added to the long-term state $\bc_{t}$ while the output gate $\bo_{t}$ aims to learn which parts of the long-term state $\bc_{t}$ should be outputted for both $\bh_{t}$ and $\by_{t}$.
\end{itemize}

The following equation (i.e., Eq. (\ref{eq:lstm})) summarises the computing process of the four layers of an LSTM network at the time step
$t$:
\begin{align}
\bi_{t} & =\sigma\left(\bW_{xi}^{\top}\bx_{t}+\bW_{hi}^{\top}\bh_{t-1}+\bb_{i}\right)\nonumber \\
\bff_{t} & =\sigma\left(\bW_{xf}^{\top}\bx_{t}+\bW_{hf}^{\top}\bh_{t-1}+\bb_{f}\right)\nonumber \\
\bo_{t} & =\sigma\left(\bW_{xo}^{\top}\bx_{t}+\bW_{ho}^{\top}\bh_{t-1}+\bb_{o}\right)\nonumber \\
\bg_{t} & =\tanh\left(\bW_{xg}^{\top}\bx_{t}+\bW_{hg}^{\top}\bh_{t-1}+\bb_{g}\right)\nonumber \\
\bc_{t} & =\bff_{t}\otimes\bc_{t-1}+\bi_{t}\otimes\bg_{t}\nonumber \\
\by_{t} & =\bh_{t}=\bo_{t}\otimes\tanh(\bc_{t-1})\label{eq:lstm}
\end{align}

where $\bW_{xi}$, $\bW_{xf}$, $\bW_{xo}$ and $\bW_{xg}$ are the weight matrices from the input vector $\bx_{t}$ to each of the four layers while $\bW_{hi}$, $\bW_{hf}$, $\bW_{ho}$ and $\bW_{hg}$ are the weight matrices from the previous short-term state $\bh_{t-1}$ to each of the four layers, and $\bb_{i}$, $\bb_{f}$, $\bb_{o}$ and $\bb_{g}$ are the bias vectors to each of the four layers, respectively.
In general, the output $\by_{t}$ can be different from the short-term state $\bh_{t}$ (i.e., $\by_{t}=\phi(\bW_{hy}^{\top}\bh_{t}+\bb_{y})$)
where $\bb_{y}$ is the bias vector while $\bW_{hy}$ is the weight from $\bh_{t}$ to $\by_{t}$, and $\phi(.)$ is the activation function (e.g., the softmax function).

\begin{figure}[h]
\begin{centering}
\includegraphics[width=0.95\columnwidth]{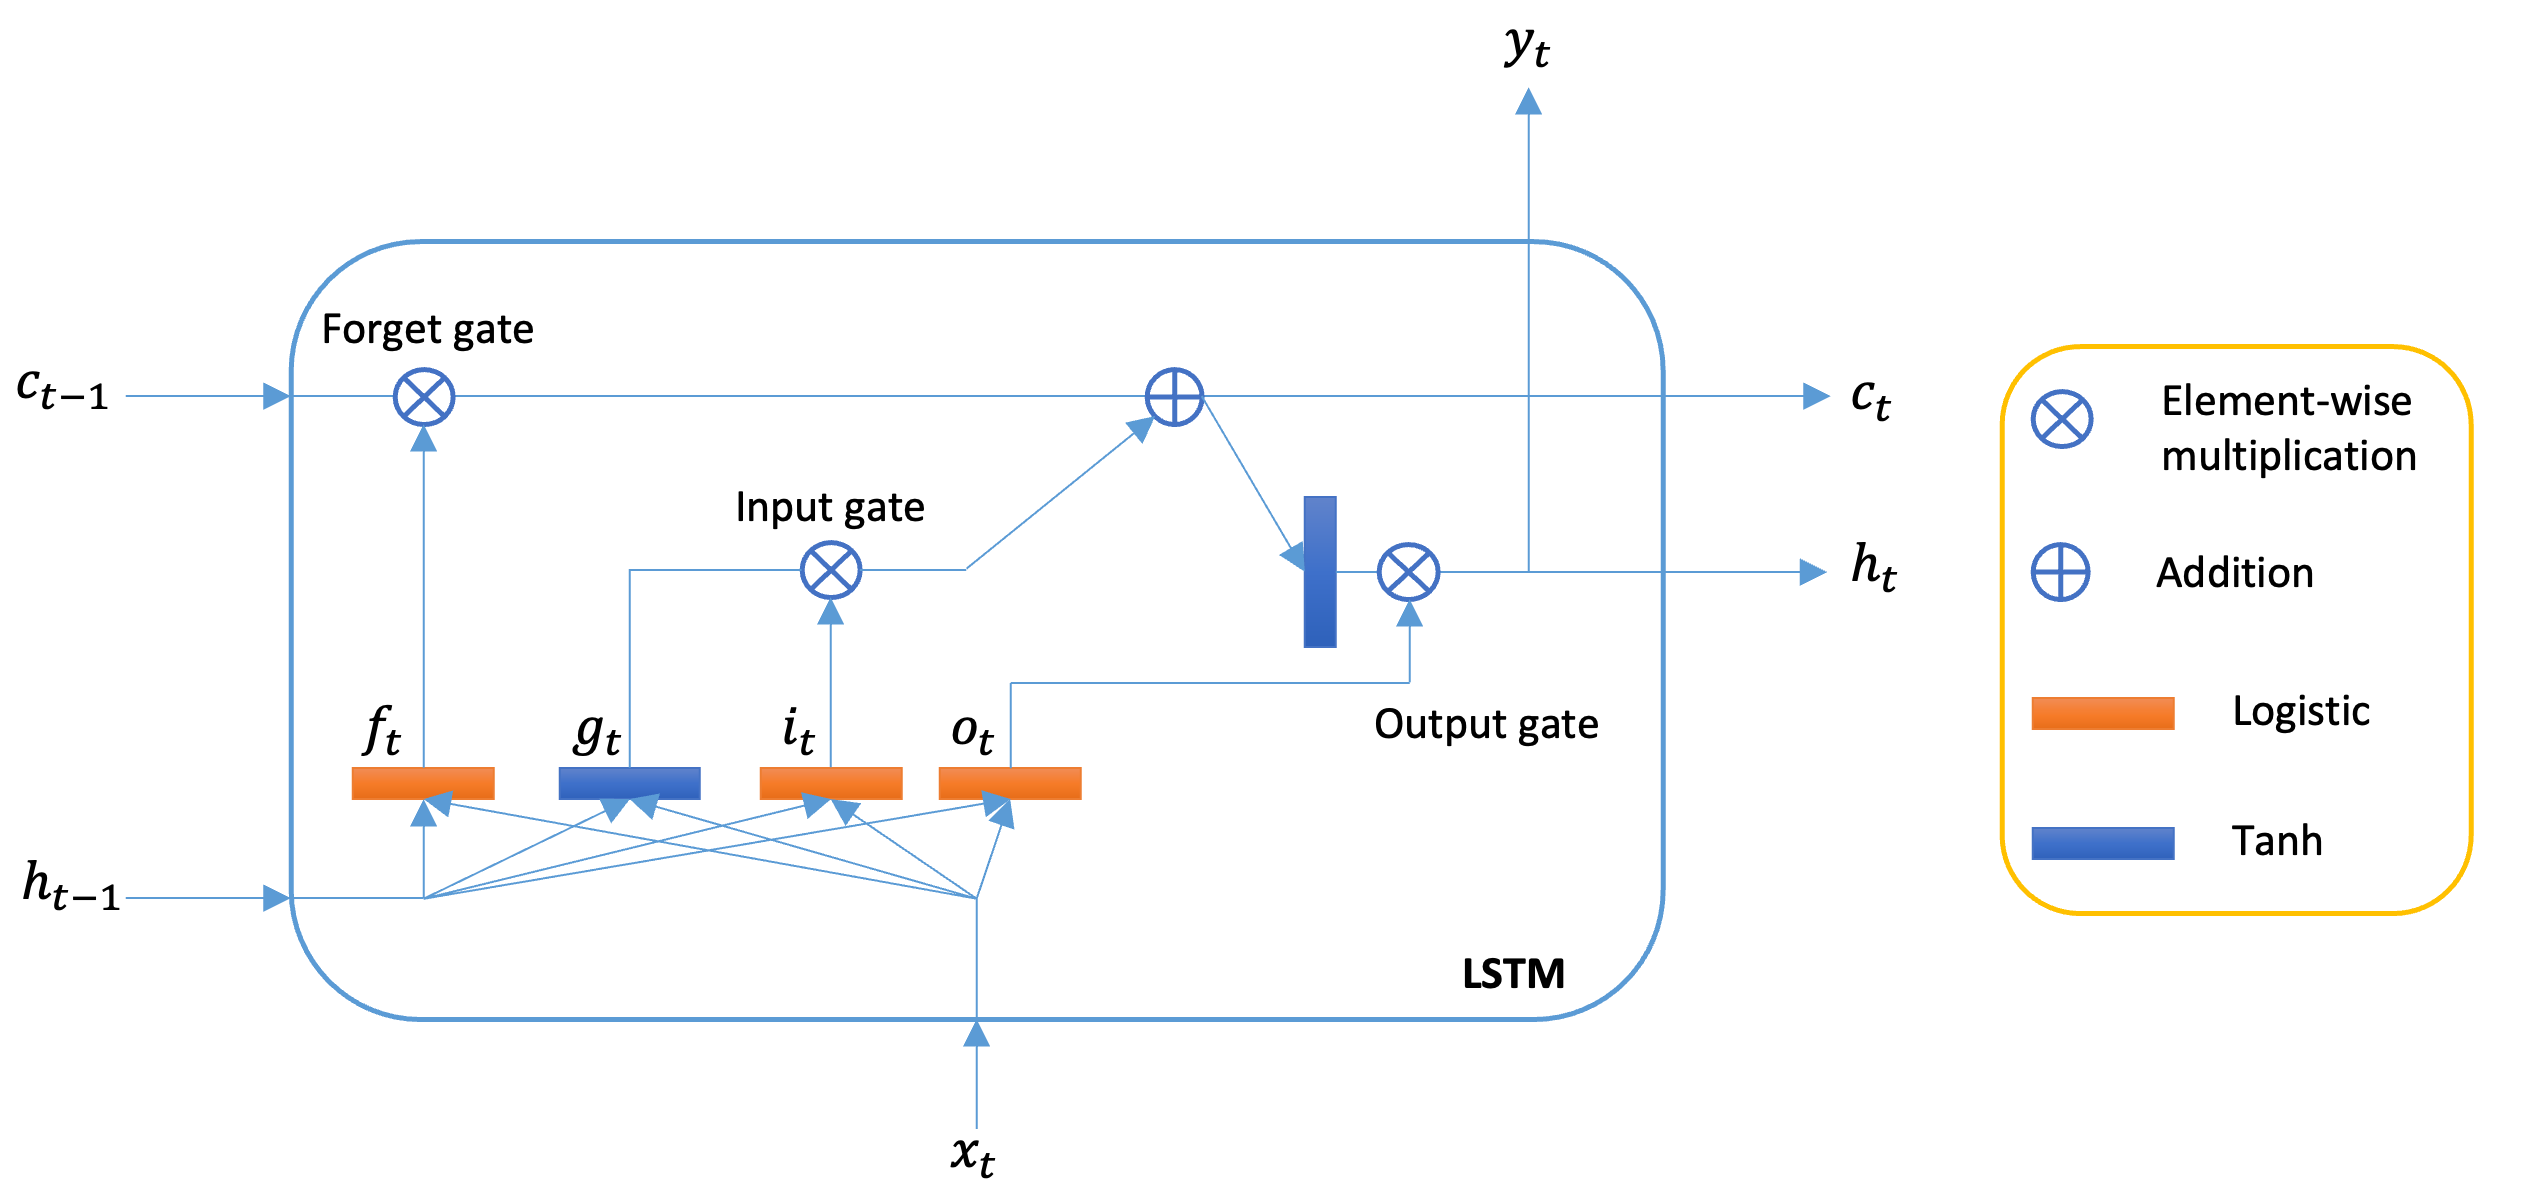}
\par\end{centering}
\caption{An architecture of a long short-term memory (LSTM) network. \label{fig:architecture-of-lstm}}
\end{figure}

\subsubsection{\textbf{Convolutional neural networks}}

Convolutional neural networks (CNNs) \cite{Lecun98gradient-basedlearning} are a kind of DNNs that are specialized for processing image data. CNNs have achieved breakthrough performance on many complex visual tasks \cite{alex_2012, TranBFTP15} such as visual object recognition, self-driving cars, automatic video classification systems, and more.
CNNs also successfully show high performance on other tasks such as voice recognition and natural language processing (NLP). In 1998, Lecun et al. \cite{Lecun98gradient-basedlearning}
introduced a typical famous architecture of a CNN named LeNet-5 as depicted in Figure \ref{fig:architecture-of-cnn}. This architecture shows some common building blocks often used in CNNs including fully
connected layers (i.e., as used in DNNs), convolutional layers, and pooling layers.

\begin{figure}[h]
\begin{centering}
\includegraphics[width=0.96\columnwidth]{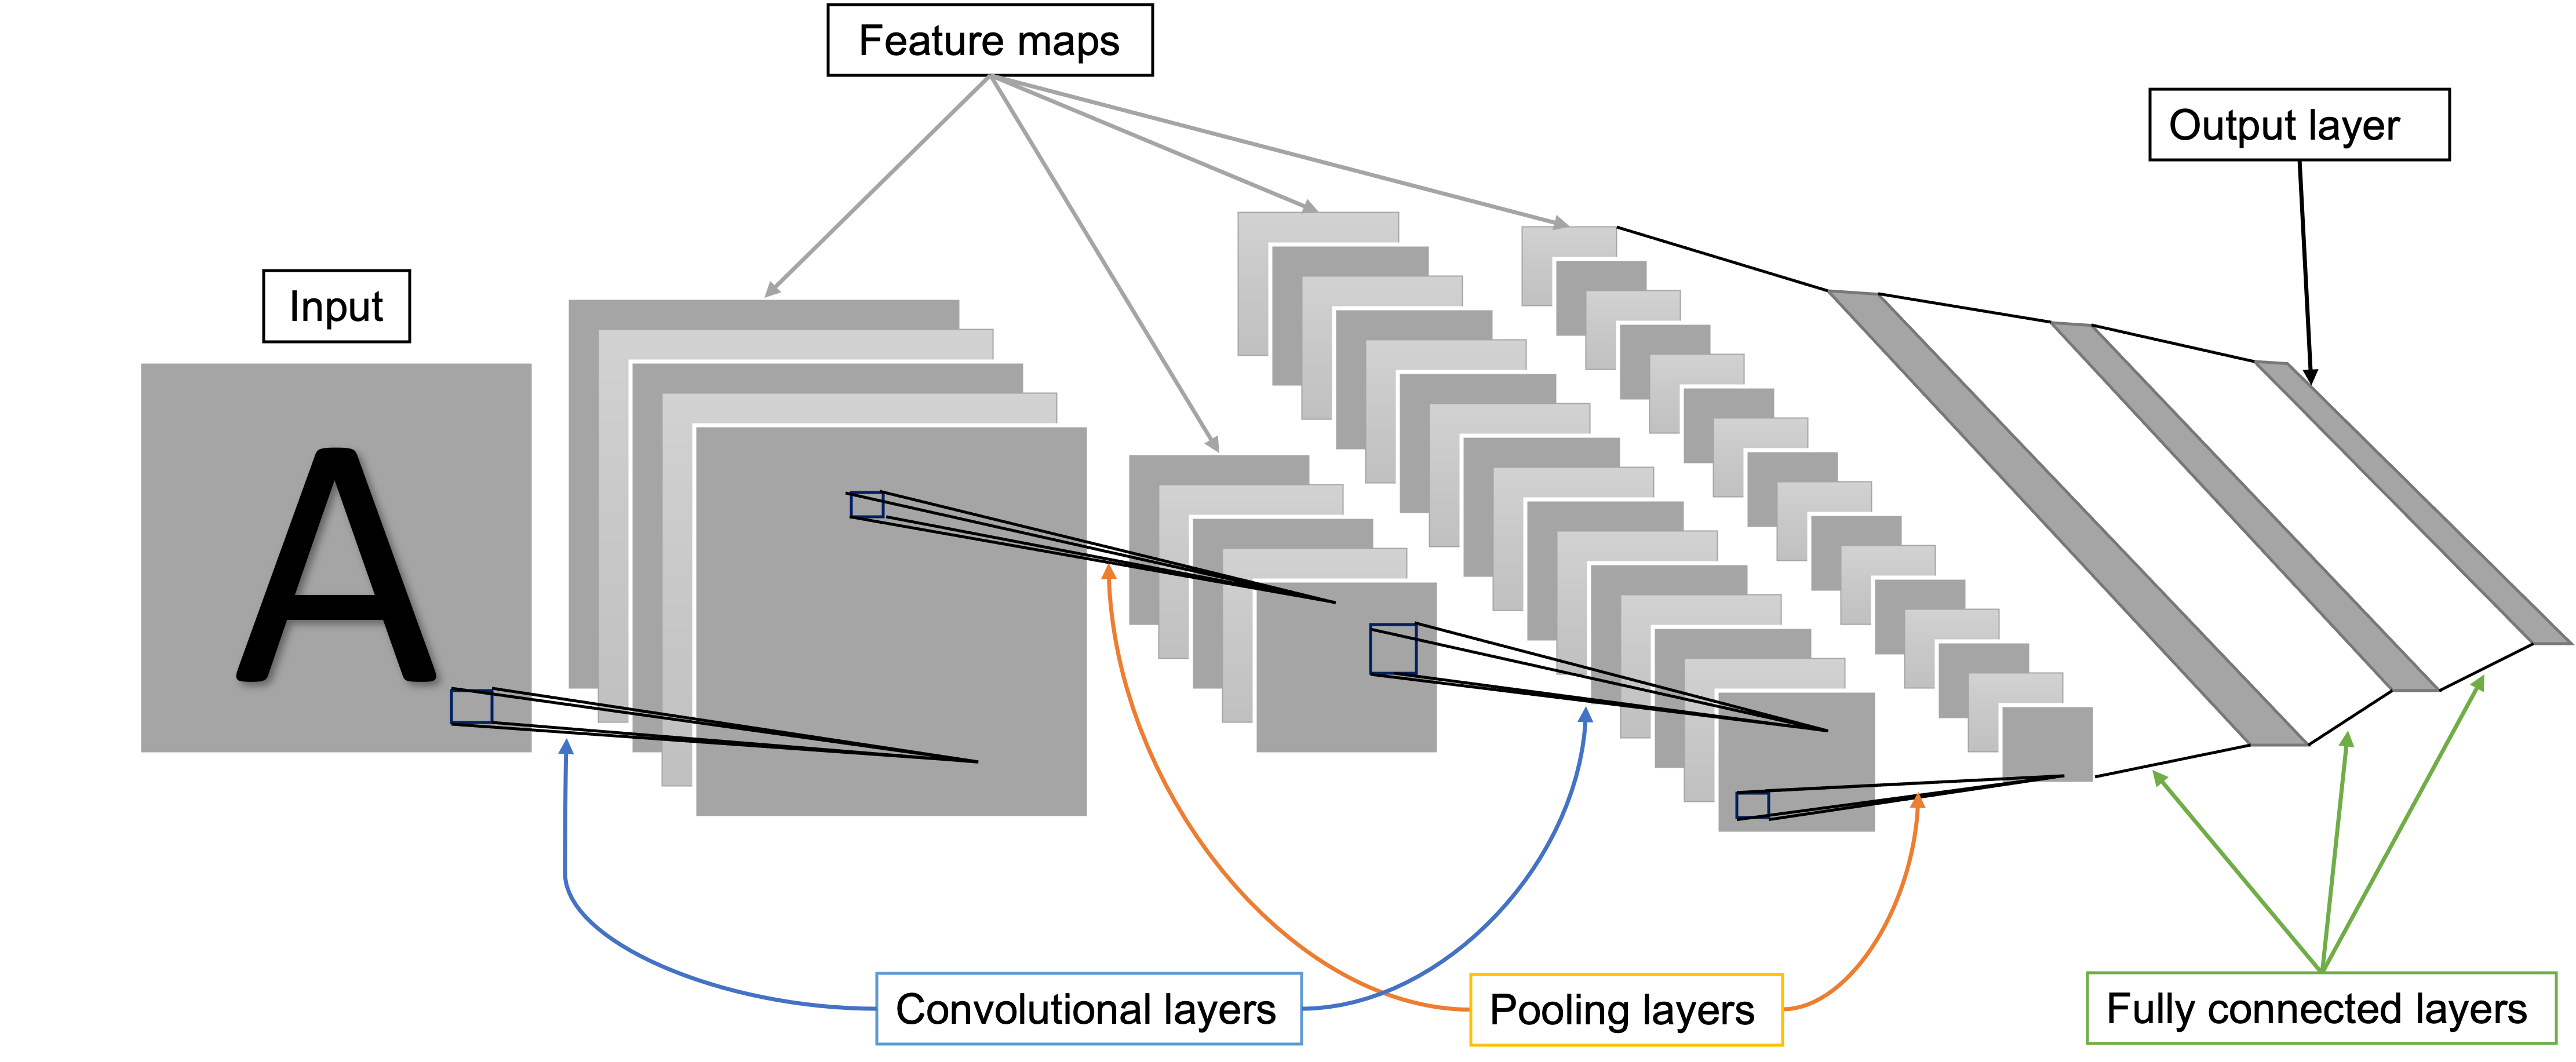}
\par\end{centering}
\caption{An architecture of LeNet-5 (a convolutional neural network) with some building blocks including convolutional layers, pooling layers, and fully connected layers. \label{fig:architecture-of-cnn}}
\end{figure}

\textbf{Convolutional layers} as shown in Figure \ref{fig:architecture-of-cnn} are the most important part of a CNN. The neurons in the first convolutional layer are connected to pixels in small rectangles (i.e., the receptive fields) of the input layer. This principle is kept for the connection between other layers (e.g., the connection between the second convolutional layer and the first convolutional layer). The neurons in the second convolutional layer are also connected to only some neurons in the first convolutional layer in the receptive fields. This architecture allows the network to concentrate on small low-level (i.e., general) features in some first hidden layers, and then assemble them into larger higher-level (i.e., specific) features in some next hidden layers. In reality, a convolutional layer often applies multiple \textbf{filters} (i.e., trainable filters and each filter outputting one feature map) to gain multiple corresponding \textbf{feature maps}, making the convolutional layer capable of detecting multiple features from its inputs.

We can summarise the computational process of convolutional layers by using Eq. (\ref{eq:cnn}) to further demonstrate how to compute the output of a given neuron
of a convolutional layer.

\begin{equation}
o_{i,j,k}=b_{k}+\sum_{u=0}^{f_{h}-1}\sum_{v=0}^{f_{w}-1}\sum_{k'=0}^{f_{k'}-1}o'_{i\times s_{h}+u,j\times s_{w}+v,k'}\times w_{u,v,k',k}\label{eq:cnn}
\end{equation}

where 
\begin{itemize}
\item $o_{i,j,k}$ is the output in row $i$ and column $j$ in the feature map $k$ of convolutional layer $l$.
\item $o'_{i\times s_{h}+u,j\times s_{w}+v,k'}$ is the output in row $i\times s_{h}+u$
and column $j\times s_{w}+v$ in the feature map $k'$ of the previous
convolutional layer $l-1$.
\item $w_{u,v,k',k}$ is the connection weight (i.e., it is updated during the training process) between any neuron in the feature map $k$ of convolutional layer $l$ and its inputs in row $u$ and column $v$ of the corresponding receptive field and feature map $k'$ of the
previous convolutional layer $l-1$ while $b_{k}$ is the bias of
the feature map $k$ of convolutional layer $l$.
\end{itemize}

The next important blocks of a CNN are pooling layers. The main goal of the \textbf{pooling layers} is to subsample (i.e., shrink) the input convolutional layer in order to reduce the computational cost. Pooling layers not only reduce memory usage but also reduce the number of parameters, thus eliminating the risk of overfitting. Pooling layers have no weights and they only aim to aggregate the inputs using an aggregation function such as the max or mean. We also need to define the size, the stride, and the padding type (i.e., zero padding or no padding) for the pooling layers.

It is worth noting that convolutional neural networks (CNNs) \cite{Lecun98gradient-basedlearning} were introduced and specialized for processing image data; However, they have also shown excellent performance when working on sequential data (e.g., text used in sentiment analysis \cite{Kim14f, ZhangW15b}).

\subsubsection{Transformers}

Transformer models \cite{transformers-Vaswani17, chatgpt} represent groundbreaking advancements in natural language processing and machine learning. These models have revolutionized various fields by demonstrating remarkable abilities in understanding and generating human-like text. Operating on a \textbf{self-attention mechanism}, transformers are uniquely adept at capturing contextual relationships in language, making them exceptionally proficient in natural language processing tasks such as language translation and text generation.

The architecture of a Transformer's framework is depicted in Figure \ref{fig:architecture-of-transformer}. In general, a Transformer follows the encoder-decoder structure used in neural sequence transduction models \cite{SutskeverVL14, Bahdanau15}. The encoder aims to map an input sequence of token representations $X=(\mathbf{x}_1,...,\mathbf{x}_n)$ to a sequence of continuous representations $Z=(\mathbf{z}_1,...,\mathbf{z}_n)$. Given $Z$, the decoder then generates an output sequence $Y=(\mathbf{y}_1,...,\mathbf{y}_n)$ of symbols one element at a time. At each step the model is auto-regressive \cite{Graves13}, consuming the previously generated tokens as additional input when generating the next token.

The encoder and decoder of a Transformer consist of multiple layers including multi-head attention layers and feed-forward neural networks. The main part of multi-head attention layers is the scaled dot product attention which is the core concept behind self-attention. In self-attention, each sequence element provides a key, value, and query. For each element, we perform an attention layer where based on its query, we check the similarity of all sequence elements’ keys and return a different, averaged value vector for each element.

\paragraph{\textbf{Scaled dot product attention}}

The core concept behind self-attention is the scaled dot product attention whose goal is to have an attention mechanism with which any element in a sequence can attend to any other while still being efficient to compute.

The dot product attention takes as input a set of queries $Q\in R^{L\times d_{k}}$, keys $K\in R^{L\times d_{k}}$, and values $V\in R^{L\times d_{v}}$ where $L$ is the sequence length and $d_{k}$ and $d_{v}$ are the hidden dimensionality for queries, keys, and values, respectively. The attention value from element $i$ to $j$ is based on its similarity of the query $Q_i$ and key $K_j$, using the dot product as the similarity metric. In math, we calculate the dot product attention as follows:

\[
Attention(Q,K,V)=softmax(\frac{QK^{T}}{\sqrt{d_{k}}})V
\]

where ${1}/{\sqrt{d_k}}$ is the scaling factor. The matrix multiplication $QK^{T}$ performs the dot product for every possible pair of queries and keys, resulting in a matrix of the shape $L\times L$. Each row represents the attention logits for a specific element to all other elements in the sequence. On these, we apply a softmax and multiply with the value vector to obtain a weighted mean (the weights being determined by the attention).

\paragraph{\textbf{Multi-Head Attention}}

The scaled dot product attention allows a network to attend over a sequence. However, often there are multiple different aspects a sequence element wants to attend to, and a single weighted average is not a good option for it. This is why the authors extend the attention mechanisms to multiple heads, i.e. multiple different query-key-value triplets on the same features. Specifically, given a query, key, and value matrix, we transform those into sub-queries, sub-keys, and sub-values, which we pass through the scaled dot product attention independently. Afterward, we concatenate the heads and combine them with a final weight matrix. Mathematically, we can express this operation as:

\begin{align*}
Multihead(Q,K,V) & =Concat(head_{1},...,head_{d})W^{O}\\
where\,\,head_{i} & =Attention(QW_{i}^{Q},KW_{i}^{K},VW_{i}^{V})
\end{align*}

In this multi-head attention computational process, $W_{1...h}^{Q}\in R^{D\times d_{k}}$, $W_{1...h}^{K}\in R^{D\times d_{k}}$,
$W_{1...h}^{V}\in R^{D\times d_{v}}$, and $W_{1...h}^{O}\in R^{h.d_{v}\times d_{out}}$ ($D$ being the input dimensionality) are the learnable parameters.

\begin{figure}[h]
\begin{centering}
\includegraphics[width=0.8\columnwidth]{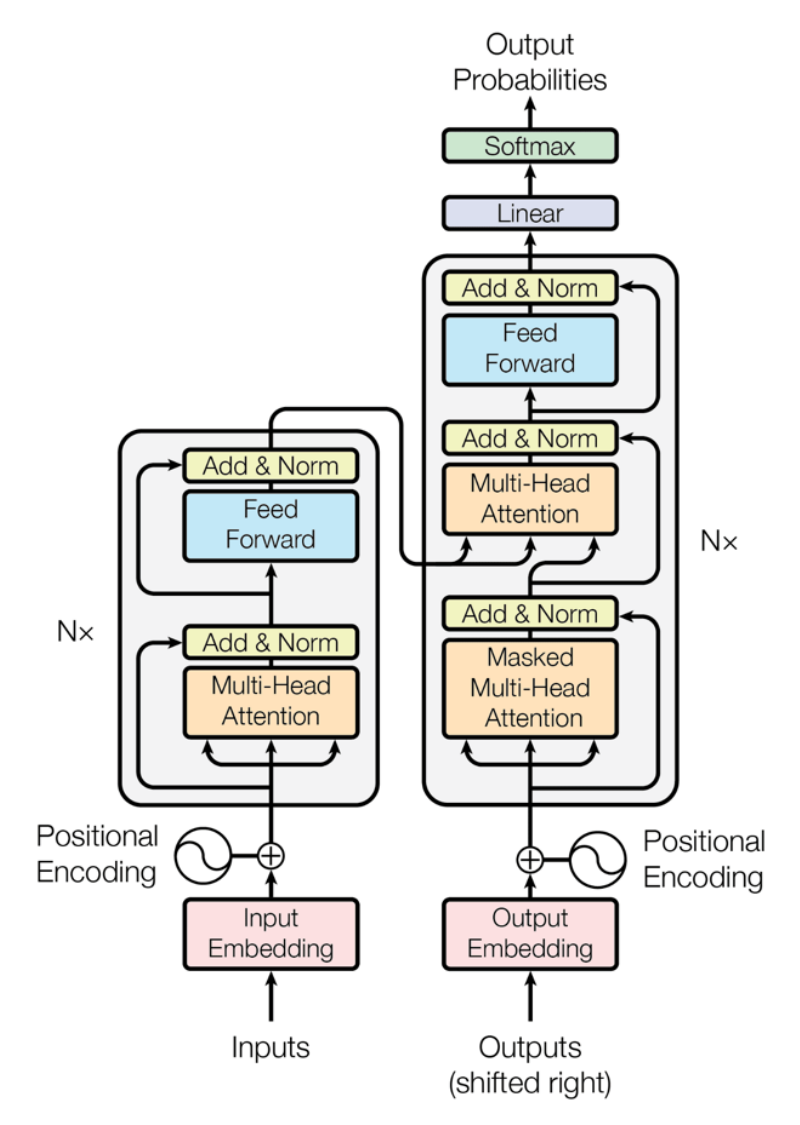}
\par\end{centering}
\caption{An architecture of the Transformer model \cite{transformers-Vaswani17}. \label{fig:architecture-of-transformer}}
\end{figure}

\subsubsection{\textbf{Graph neural networks}}

A Graph Neural Network (GNN) is a powerful deep learning architecture designed to analyze and process data represented in the form of graphs. GNNs are specialized in capturing complex relationships and interactions within interconnected nodes. They operate by propagating information through the graph's nodes and edges, allowing them to learn patterns and features from both local and global contexts. GNNs have found applications in diverse fields such as social network analysis, recommendation systems, molecular chemistry, and spatial data analysis, demonstrating their versatility in addressing real-world problems involving interconnected data points.

A graph is represented as $G=(V, E)$ where $V$ is the set of vertices (or nodes), and $E$ is the set of edges. Let $v_i \in V$ to denote a node and $e_{ij} = (v_i, v_j) \in E$ to denote an edge pointing from $v_i$ to $v_j$. The neighborhood of a node $v$ is defined as $N(v) = \{u \in V | (u, v) \in E \}$. The adjacency matrix $A$ is a $n \times n$ matrix with $A_{ij}=1$ if $e_{ij} \in E$ and $A_{ij}=0$ if $e_{ij} \notin E$. A graph may have node attributes $X$, where $X \in R^{n \times d}$ is a node feature matrix with $x_v \in R^{d}$ representing the feature vector of a node $v$. Meanwhile, a graph may have edge attributes $X^e$, where $X^e \in R^{m \times c}$ is an edge feature matrix with $x_{v,u}^{e}\in R^{c}$ representing the feature vector of an edge $(v, u)$.

One popular category of GNNs is Convolutional graph neural networks (ConvGNNs) which generalize the operation of convolution from grid data to graph data. The main idea is to generate a node $v$’s representation by aggregating its own features $x_v$ and neighbors’ features $x_u$, where $u \in N(v)$. Particularly, ConvGNNs stack multiple graph convolutional layers to extract high-level node representations. ConvGNNs play a central role in building up many other complex GNN models. Figure \ref{fig:architecture-of-ConvGNN} shows a ConvGNN with multiple graph convolutional layers for nodes' representation learning.

We consider a multi-layer Graph Convolutional Network (GCN) with the following layer-wise propagation rule:

\[
H^{(l+1)}=\sigma(\tilde{D}^{-1/2}\tilde{A}\tilde{D}^{-1/2}H^{(l)}W^{(l)})
\]

Here, $\tilde{A}=A+I_{N}$ is the adjacency matrix of the undirected graph $G$ with added self-connections. $I_{N}$ is the identity matrix,
$\tilde{D}_{ii}=\sum_{j}\tilde{A}_{ij}$ and $W^{(l)}$ is a layer-specific trainable weight matrix. $\sigma(.)$ denotes an activation function, such as the $RELU(.)=max(0,.)$. $H^{(l)}\in R^{N\times D}$ is the matrix of activations in the $l^{th}$ layer with $H^{(0)}=X$.

\begin{figure}[h]
\begin{centering}
\includegraphics[width=0.88\columnwidth]{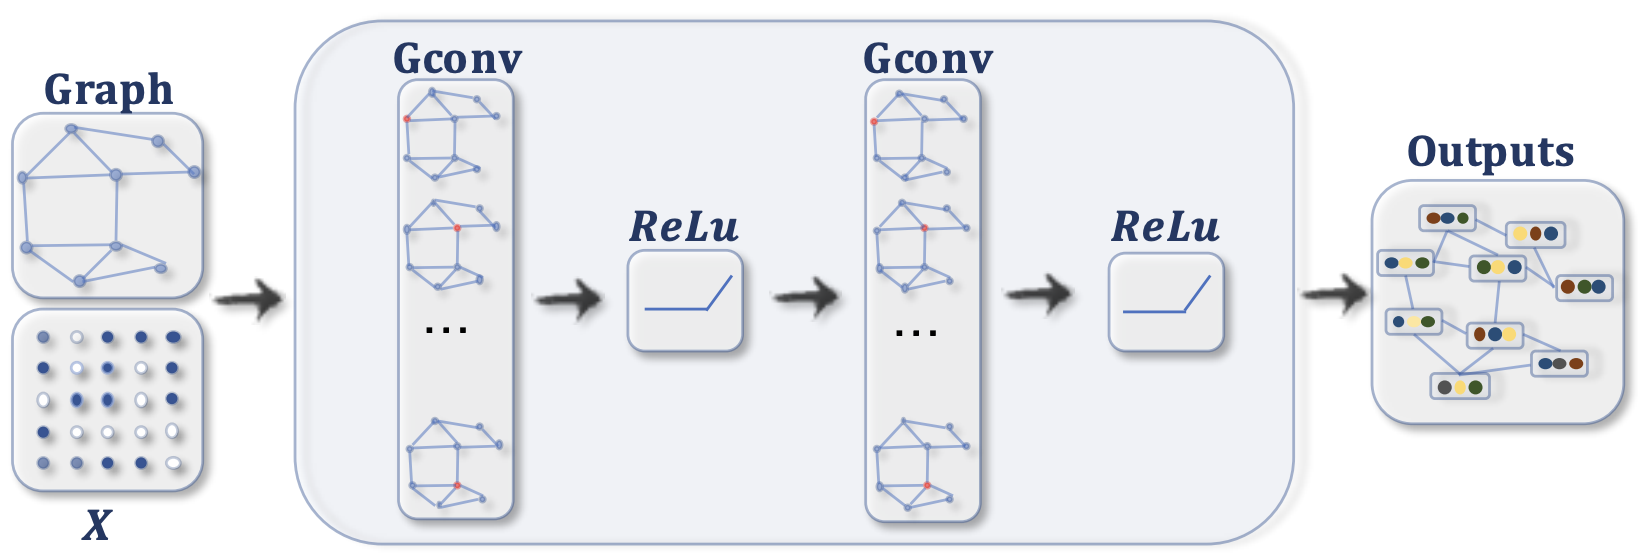}
\par\end{centering}
\caption{A ConvGNN with multiple graph convolutional layers. A graph convolutional layer captures the underlying representation of each node by aggregating feature information from its neighborhood nodes. Following this aggregation, a non-linear transformation is applied to the resulting outputs. By stacking multiple layers, the final representation of each node receives messages from its neighborhood. \label{fig:architecture-of-ConvGNN}}
\end{figure}

Please refer to \cite{GNNssurveys} for the details of other categories of graph neural networks (GNNs) including Recurrent graph neural networks (RecGNNs), Graph autoencoders (GAEs), and Spatial-temporal graph neural networks (STGNNs).

\subsubsection{\textbf{Mahalanobis distance}}

A rich line of machine learning and deep learning algorithms has been developed for out-of-distribution (OOD) detection, among which distance-based methods demonstrated promise \cite{lee2018simple, Tack2020, Sehwag21}. Distance-based methods leverage feature embeddings extracted from a model and operate under the assumption that the test OOD samples are relatively far away from the ID data. For example, \cite{Sehwag21} uses the Mahalanobis distance \cite{Mahalanobis} to all cluster centroids for OOD detection. In particular, the authors first partition the features for in-distribution training data in $M$ clusters. They represent features for each cluster as $Z_m$ (by using the k-means clustering method due to its effectiveness and low computation cost). Next, they model features in each cluster independently and calculate the following $outlier\, score(s_{\mathbf{x}})=min_{m}D(\mathbf{x}, Z_{m})$ for each test input $\mathbf{x}$, where $D(., .)$ is a distance metric in the feature space. The Mahalanobis distance to calculate the outlier score of each input data $x$ in the latent space is as follows:

\[
s(x)=min_{k}(\mathbf{z}_\mathbf{x}-\mu_{m})^{\mathrm{\top}}\Sigma_{m}^{-1}(\mathbf{z}_\mathbf{x}-\mu_{m})
\]

where $\mathbf{z}_\mathbf{x}$ is the representation of data $\mathbf{x}$ in the latent space while $\mu_{m}$ and $\Sigma_{m}$ are the sample mean and sample covariance of cluster $m^{th}\in M$.

\subsubsection{\textbf{Contrastive loss functions}}

Using contrastive loss functions for improving data representations has been widely applied to computer vision domain applications from computer vision classification, detection, and segmentation \cite{NEURIPS2020_Kim, Wang_2021_ICCV, Sun_2021_CVPR, Du_2022_CVPR, Wang_2021_CVPR} to vision data out-of-distribution detection \cite{Sehwag21}.

\paragraph{\textbf{Self-supervised contrastive learning}}

For a set of $N$ randomly sampled sample and label pairs, $\{\mathbf{x}_k, y_k\}_{k=1...N}$, the corresponding batch used for training consists of $2N$ pairs, $\{\tilde{\mathbf{x}}_l, \tilde{y}_l\}_{l=1...2N}$, where $\tilde{\mathbf{x}}_{2k}$ and $\tilde{\mathbf{x}}_{2k-1}$ are two random augmentations of $\mathbf{x}_k (k=1...N)$ and $\tilde{y}_{2k-1}=\tilde{y}_{2k} = y_k$. We refer to a set of $N$ samples as a “batch” and the set of 2N augmented samples as a “multi-viewed batch”.

Within a multi-viewed batch, let $i\in I \equiv \{1...2N\}$ be the index of an arbitrary augmented sample, and let $j(i)$ be the index of the other augmented sample originating from the same source sample.
In self-supervised contrastive learning (SimCLR), the loss takes the following form:

\[
\mathcal{L}^{self}=\sum_{i\in I}\mathcal{L}_{i}^{self}=-\sum_{i\in I}log\frac{exp(sim(\mathbf{z},\mathbf{z}_{j(i)})/\tau)}{\sum_{\alpha\in A(i)}exp(sim(\mathbf{z},\mathbf{z}_{a})/\tau)}
\]

where $\mathbf{z}_{l}$ can be considered as a representation of corresponding $\mathbf{x}$; $sim$ function can be the inner (dot) product; $\tau\in R^{+}$ is a scalar temperature parameter, and $A(i) \equiv I\setminus{i}$. The index $i$ is called the anchor, index $j(i)$ is called the positive, and the other $2(N-1)$ indices ($\{k \in A(i) \setminus \{j(i)\}\})$ are called the negatives. Note that for each anchor $i$, there is one positive pair and $2N-2$ negative pairs. The denominator has a total of $2N-1$ terms (the positives and negatives).

\paragraph{\textbf{Supervised contrastive learning}}
Supervised contrastive learning (SupCLR) is a supervised version of self-supervised contrastive learning (SimCLR). That builds on the contrastive self-supervised literature by leveraging label information. Normalized embeddings from the same class are pulled closer together than embeddings from different classes:

\[
\mathcal{L}^{sup}=\sum_{i\in I}\mathcal{L}_{i}^{sup}=\sum_{i\in I}\frac{-1}{\left|P(i)\right|}log\frac{exp(sim(\mathbf{z},\mathbf{z}_{p})/\tau)}{\sum_{\alpha\in A(i)}exp(sim(\mathbf{z},\mathbf{z}_{a})/\tau)}
\]

where $P(i) \equiv \{p \in A(i): \tilde{y}_p = \tilde{y}_i\}$ is the set of indices of all positives in the multi-viewed batch distinct from $i$, and $\left|P(i)\right|$ is its cardinality.

\subsubsection{\textbf{Cosine similarity}}\label{sec:cosines}

Cosine similarity is a metric used to measure the similarity of two vectors. In particular, cosine similarity measures the similarity in the direction or orientation of the vectors ignoring differences in their magnitude or scale. The similarity of two vectors is measured by the cosine of the angle between them (please refer to Figure \ref{fig:cosine-similarity} for details). In our paper, to form the corresponding vector for each $\tilde{X}$ of each source code section $X$ in the latent space for calculating the cosine similarity, we simply concatenate all vectors where each vector stands for a representation of a code statement in $\tilde{X}$.

\subsubsection{\textbf{Mutual information}}

Mutual information (MI) is used to measure the dependence
between two random variables \cite{TheoryofC, EofIT2006}. It captures how much the knowledge of one random variable reduces the uncertainty of the other. In particular, MI quantifies the amount of information obtained about one random variable by observing the other random variable. For example, consider a scenario where variable A denotes the outcome of rolling a standard 6-sided die and variable B represents whether the roll results in an even number (0 for even, 1 for odd). Evidently, the information conveyed by B provides insights into the value of A, and vice versa. In other words, these random variables possess mutual information.

Assume that we have two random variables $X$ and $Y$ drawn from the joint distribution $p(x,y)$ with two corresponding marginal distributions $p(x)$ and $p(y)$. The mutual information between $X$ and $Y$ denoted by $I(X,Y)$ is the relative entropy between the joint distribution $p(x,y)$ and the product distribution $p(x)p(y)$, and is defined as follows:

{
\begin{align}
    I(X,Y)= & \sum_{x\in\mathcal{X}}\sum_{y\in\mathcal{Y}}p(x,y)\log\frac{p(x,y)}{p(x)p(y)} \nonumber \\ = & D_{KL}(p(x,y)||p(x)p(y))
\end{align}
}

where $D_{KL}(p(x,y)||p(x)p(y))$ is the Kullback-Leibler divergence measuring the relative entropy (i..e, the difference in information) represented by two distributions, i.e., the product of marginal distributions $p(x)p(y)$ of $X$ and $Y$ from their joint distribution $p(x,y)$.

\subsubsection{\textbf{Information bottlenecks}}

Here, we consider the supervised learning context where we want to predict corresponding outputs (e.g., labels) $\left\{ \by_{i}\right\} _{i=1}^{n}$ of given inputs $\left\{ \bx_{i}\right\} _{i=1}^{n}$. A deep learning network (DNN) will learn latent representations (i.e., latent features in the latent space that contain useful information to describe the data) $\left\{ \tilde{\bx}_{i}\right\} _{i=1}^{n}$ of the corresponding input data samples $\left\{ \bx_{i}\right\} _{i=1}^{n}$ in terms of enabling good predictions and generalizations.

Assume that the whole hidden layer in Figure \ref{fig:Bottneck_theory} is denoted by a random variable $\tilde{X}$ while the input and output layers are denoted by random variables $X$ and $Y$ respectively. We can describe this hidden layer by two conditional distributions: the encoder $p(\tilde{\bx}|\bx)$ and the decoder $p(\by|\tilde{\bx})$. This transformation process preserves the information of the input layer $X$ without considering which individual neurons within the hidden layer $\widetilde{X}$ encode which features (i.e., neurons) of $X$. An optimal encoder process of the mutual information between $X$ and the desired output $Y$ denoted by $I(X,Y)$ can create the most compact encoding (i.e., minimally sufficient statistic) $\tilde{X}$ of the input data $X$ while $\tilde{X}$ still has enough information (i.e., $\tilde{X}$ can capture the important features of $X$ as well as remove the unnecessary parts of $X$ that do not make any contributions to the prediction of $Y$) to predict $Y$ as accurately as possible.

An information bottleneck \cite{tishby2000information,tishby2015deep}
is proposed to be a computational framework that aims to find the most compact encoding $\tilde{X}$ of the input data $X$. In particular, it is the optimal trade-off between the compression $\tilde{X}$ and the prediction of the desired output $Y$ as described in the following optimization problem:
\begin{equation}
\min_{p(\tilde{\bx}|\bx),p(\by|\tilde{\bx}),p(\tilde{\bx})}\left\{ I(X,\tilde{X})-\beta I(\tilde{X},Y)\right\} \label{eq:information-bottleneck}
\end{equation}

where $\beta$ specifies the amount of relevant information captured by the encoding process (i.e., the representations $\tilde{X}$ and $I(\tilde{X}, Y)$).

\begin{figure}[h]
\begin{centering}
\includegraphics[width=0.5\columnwidth]{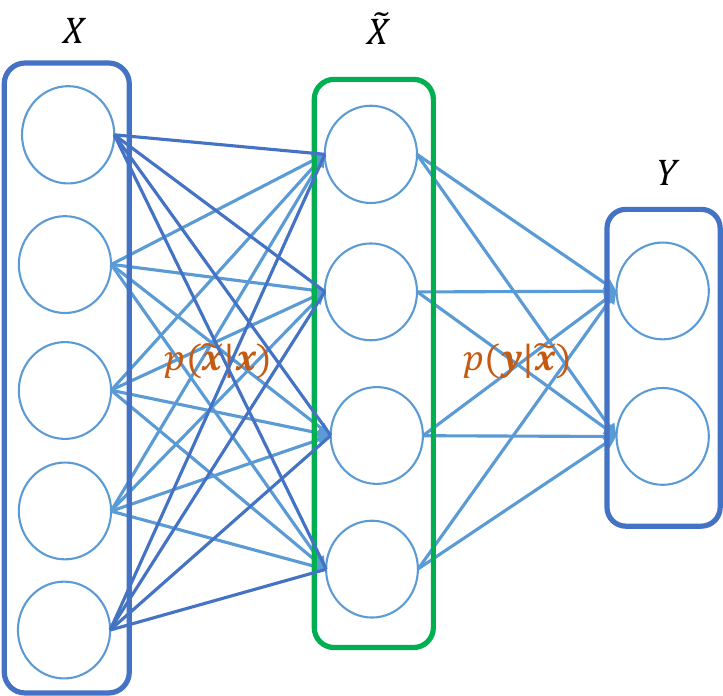}
\par\end{centering}
\vspace{-1mm}
\caption{An architecture of a simple deep neural network in a supervised learning context for the classification problem. \label{fig:Bottneck_theory}}
\end{figure}

\begin{figure*}[t]%
\begin{centering}
%\vspace{-1mm}
\begin{tabular}{c}
\includegraphics[width=0.9\textwidth]{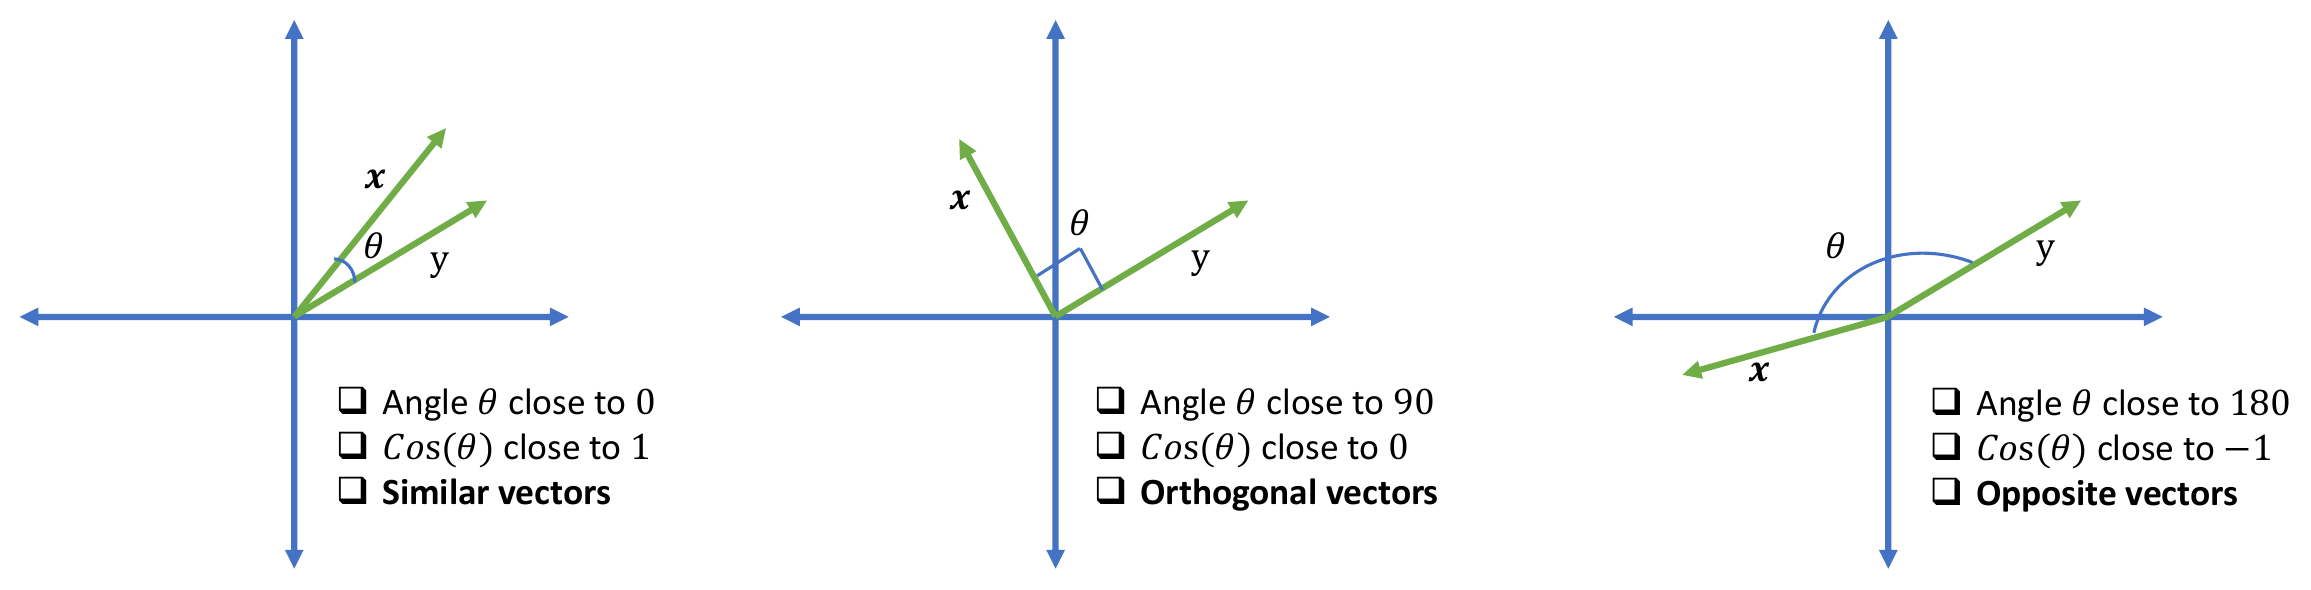}\tabularnewline
\end{tabular}\vspace{-1mm}
\par\end{centering}
\caption{A graphic showing two vectors with cosine similarities close to 1, close to 0, and close to -1. The similarity of two vectors is measured by the cosine of the angle between them. The similarity can take values between -1 and +1. Smaller angles between vectors produce larger cosine values, indicating greater cosine similarity.\label{fig:cosine-similarity}}
\vspace{-3mm}
\end{figure*}%
