# Supplementary material for: Deep Learning-Based Out-of-distribution Source Code Data Identification: How Far Have We Gone?
Source: arXiv:2404.05964 source file (2024-04-15)
Supplement: Supplementary file 2 [file appendix.tex]

\section{Appendix}\label{sec:appendix}

\subsection{Data processing and embedding\label{sec:datape}}

We preprocessed the datasets before injecting them into deep neural networks. In particular, we standardized the source code by (i) removing comments, blank lines, and non-ASCII characters, and (ii) mapping user-defined variables to symbolic variable names (e.g., \emph{var1} and \emph{var2}) and user-defined
functions to symbolic function names (e.g., \emph{func1} and \emph{func2}) using Treesitter \cite{Treesitter}.  We also replaced strings with a generic \emph{"str"} token.

We then embedded source code statements into vectors. For instance, consider the following statement (C/C++ programming language) \emph{"for(var1=0;var1<10;var1++)"}, we use the byte pair encoding (BPE) algorithm \cite{sennrich2016neural} (i.e., commonly used in large language models, e.g., CodeBERT \cite{CodeBERT2020} for tokenization) to tokenize this statement into a sequence of tokens, and then we used a 150-dimensional token Embedding layer followed by a Dropout layer with a dropped fixed probability $p=0.2$ and (a 1D convolutional layer with the filter size $150$ and kernel size $3$, and a 1D max pooling layer) or (a 1D max pooling layer) to encode each statement in a function $F$. Finally, a mini-batch of functions in which each function consisting of $L$ encoded statements was fed to the deep learning-based models. Note that the Embedding and convolutional layers are learnable during the training process.

It is worth noting that the length ($L$) of each function is padded or truncated to $100$ source code statements  (i.e., we base on the quantile values of the source code data’ length of the used datasets to decide the length of each source code data sample). Furthermore, we observe that almost all important information relevant to the vulnerability of each source code data sample (e.g., a function) lies in the first $100$ code statements.

\subsection{Model's configurations}\label{sec:modelc}

For the main baselines of our \textbf{\ourapp~}method including \textbf{Standard DNN} \cite{Hendrycks2017dnn}, \textbf{Outlier Exposure} \cite{Hendrycks18}, and \textbf{SSD} \cite{Sehwag21}. These methods are popular and state-of-the-art approaches for out-of-distribution detection applied in the computer vision domain. To make them applicable for out-of-distribution source code vulnerability detection, we keep the principle of these methods and use the same data embedding process for handling the sequential source code data as used in our method. For the popular and state-of-the-art baselines (i.e., \textbf{VulDeePecker} \cite{VulDeePecker2018}, \textbf{CodeBERT} \cite{CodeBERT2020}, and \textbf{ReGVD} \cite{ReGVD2022}) in the software vulnerability detection problem, we use the architecture proposed in the corresponding original papers.

To our \ourapp~ method, for the $g\left(\cdot;\alpha\right)$
and $f\left(\cdot;\beta\right)$ networks, we used deep feed-forward neural networks having three and two hidden layers with the size of each hidden layer in $\left\{100,300\right\} $. The dense hidden layers are followed by a ReLU function as nonlinearity and Dropout \cite{srivastava14a} with a retained fixed probability $p=0.8$ as regularization. The last dense layer of the $g\left(\cdot;\alpha\right)$ network for learning a discrete distribution is followed by a sigmoid function while the last dense layer of the $f\left(\cdot;\beta\right)$ network is followed by a softmax function for predicting. The number of chosen clusters guiding the computation of the innovative cluster-contrastive learning mentioned is from $2$ to $5$ in the case of the distribution data consisting of one vulnerability type. When the in-distribution data consists of more than one vulnerability type, the number of vulnerability patterns used in cluster-contrastive learning also needs to be increased. In the cases of two or more two vulnerability types (i.e., three), we vary and tune the number of clusters in the range of $2$ to $15$.
The trade-off hyper-parameter $\lambda$ representing the weight of the innovative cluster-contrastive learning is in $\{10^{-2},10^{-1},10^{0}\}$ while the scalar temperature $\tau$ is in $\{0.5, 1.0\}$. The temperature $\nu$ for the Gumbel softmax distribution is also set in $\{0.5, 1.0\}$.

For our \ourapp~ method and baselines, we employed
the Adam optimizer \cite{KingmaB14} with an initial learning rate
equal to $10^{-3}$, while the mini-batch size is set to $128$. For the training process, we split the data of each in-distribution data set into two random partitions. The first partition contains 80\% for training, the second partition contains 20\% for validation. For each in-distribution data set, we used $10$ epochs for the training process. We additionally applied gradient clipping regularization to prevent over-fitting. For each method, we ran the corresponding model several times and reported the averaged FPR (at TPR 95\%), AUROC, and AUPR measures. We ran our experiments in Python
using Tensorflow \cite{abadi2016tensorflow} for the used methods
on a 13th Gen Intel(R) Core(TM) i9-13900KF having 24 CPU Cores at 3.00 GHz with 32GB RAM, integrated Gigabyte RTX 4090 Gaming OC 24GB. Some baseline methods (i.e., \textbf{CodeBERT} \cite{CodeBERT2020} and \textbf{ReGVD} \cite{ReGVD2022}) were written using Pytorch \cite{pytorch2019}. For these baseline methods, we followed the source code samples published by the authors.

\begin{table}[ht]
\centering{}
\resizebox{0.93\columnwidth}{!}{
\begin{tabular}{ccrrr}
\hline 
%\textbf{ID and OOD Datasets} & \textbf{Methods} & \textbf{FPR} $\downarrow$ & \textbf{AUROC} $\uparrow$ & \textbf{AUPR} $\uparrow$
\textbf{ID and OOD} & \textbf{Methods} & \textbf{FPR} $\downarrow$& \textbf{AUROC} $\uparrow$& \textbf{AUPR} $\uparrow$
\tabularnewline
\hline 
 
\multirow{7}{*}{CWE20 vs. CWE264}
&  Standard DNN & 89.58\%	& 76.48\%	& 17.40\%
\tabularnewline
%\cline{2-5} \cline{3-5} \cline{4-5} \cline{5-5} 
&  Outlier Exposure & 91.93\% &  78.86\% &  18.00\%  
\tabularnewline
%\cline{2-5} \cline{3-5} \cline{4-5} \cline{5-5} 
&  SSD & 88.28\%	& 86.27\%	& 26.44\%
\tabularnewline
%\cline{2-5} \cline{3-5} \cline{4-5} \cline{5-5} 
&  VulDeePecker & \underline{72.14\%}	& \underline{92.33\%}	& \underline{37.41\%}
\tabularnewline
%\cline{2-5} \cline{3-5} \cline{4-5} \cline{5-5} 
&  CodeBERT  & 90.31\%	& 48.86\%	& 13.21\%
\tabularnewline
%\cline{2-5} \cline{3-5} \cline{4-5} \cline{5-5} 
&  ReGVD & 91.13\%	& 63.96\%	& 15.80\%
\tabularnewline
\cline{2-5} \cline{3-5} \cline{4-5} \cline{5-5} 
&  \multirow{2}{*}{\ourapp~ (Ours)}  & \textbf{0.00\%} & \textbf{99.63\%} & \textbf{92.77\%}
\tabularnewline
%\cline{3-5} \cline{4-5} \cline{5-5} 
 &  & \textcolor{blue}{($\downarrow$ 72.14\%)} & \textcolor{blue}{($\uparrow$ 7.3\%)} & \textcolor{blue}{($\uparrow$ 55.36\%)}\tabularnewline
\hline

\multirow{7}{*}{CWE200 vs. CWE119}
&  Standard DNN & 88.02\%	& 77.84\%	& 71.74\%
\tabularnewline
%\cline{2-5} \cline{3-5} \cline{4-5} \cline{5-5} 
&  Outlier Exposure &  84.79\%	& 82.74\%	& 76.94\%
\tabularnewline
%\cline{2-5} \cline{3-5} \cline{4-5} \cline{5-5} 
&  SSD & 88.23\%	& 80.88\%	& 74.28\%
\tabularnewline
%\cline{2-5} \cline{3-5} \cline{4-5} \cline{5-5} 
&  VulDeePecker & \underline{24.58\%}	& \underline{94.60\%}	& \underline{95.49\%}
\tabularnewline
%\cline{2-5} \cline{3-5} \cline{4-5} \cline{5-5} 
&  CodeBERT  & 58.16\%	& 72.91\% & 80.98\%
\tabularnewline
%\cline{2-5} \cline{3-5} \cline{4-5} \cline{5-5} 
&  ReGVD  & 95.58\%	& 55.13\%	& 56.73\%
\tabularnewline
\cline{2-5} \cline{3-5} \cline{4-5} \cline{5-5} 
%&  \ourapp~ (Ours)  & \textbf{0.00\%} & \textbf{99.32\%} & \textbf{99.05\%}
%\tabularnewline

& \multirow{2}{*}{LEO (Ours)} & \textbf{0.00\%} & \textbf{99.32\%} & \textbf{99.05\%}\tabularnewline
%\cline{3-5} \cline{4-5} \cline{5-5} 
 &  & \textcolor{blue}{($\downarrow$ 24.58\%)} & \textcolor{blue}{($\uparrow$ 4.72\%)} & \textcolor{blue}{($\uparrow$ 3.56\%)}\tabularnewline

 \hline
\multirow{7}{*}{CWE200 vs. CWE264}
&  Standard DNN & 93.49\%	& 67.11\%	& 25.40\%
\tabularnewline
%\cline{2-5} \cline{3-5} \cline{4-5} \cline{5-5} 
&  Outlier Exposure &  91.67\%	& 75.52\%	& 31.59\%
\tabularnewline
%\cline{2-5} \cline{3-5} \cline{4-5} \cline{5-5} 
&  SSD & 87.24\%	& \underline{80.50\%}	& 37.54\%
\tabularnewline
%\cline{2-5} \cline{3-5} \cline{4-5} \cline{5-5} 
&  VulDeePecker & 65.36\%	& 74.24\%	& 53.21\%
\tabularnewline
%\cline{2-5} \cline{3-5} \cline{4-5} \cline{5-5} 
&  CodeBERT  & \underline{60.00\%}	& 70.74\%	& \underline{57.74\%}
\tabularnewline
%\cline{2-5} \cline{3-5} \cline{4-5} \cline{5-5} 
&  ReGVD  & 95.46\%	& 54.03\%	& 23.88\%
\tabularnewline
\cline{2-5} \cline{3-5} \cline{4-5} \cline{5-5} 
&  \multirow{2}{*}{\ourapp~ (Ours)}  & \textbf{0.00\%} & \textbf{99.91\%} & \textbf{99.26\%}
\tabularnewline
%\cline{3-5} \cline{4-5} \cline{5-5} 
 &  & \textcolor{blue}{($\downarrow$ 60.00\%)} & \textcolor{blue}{($\uparrow$ 19.41\%)} & \textcolor{blue}{($\uparrow$ 41.52\%)}\tabularnewline
\hline

%\hline
\multirow{7}{*}{CWE264 vs. CWE20}
&  Standard DNN & 91.80\%	& 62.03\%	& 38.20\%
\tabularnewline
%\cline{2-5} \cline{3-5} \cline{4-5} \cline{5-5} 
&  Outlier Exposure &  83.50\% &  72.09\% & 48.95\%
\tabularnewline
%\cline{2-5} \cline{3-5} \cline{4-5} \cline{5-5} 
&  SSD & 85.84\%	& 82.97\%	& 59.62\%
\tabularnewline
%\cline{2-5} \cline{3-5} \cline{4-5} \cline{5-5} 
&  VulDeePecker & 52.34\%	& 90.88\%	& 74.79\%
\tabularnewline
%\cline{2-5} \cline{3-5} \cline{4-5} \cline{5-5} 
&  CodeBERT  & \underline{10.06\%}	& \underline{95.57\%}	& \underline{95.31\%}
\tabularnewline
%\cline{2-5} \cline{3-5} \cline{4-5} \cline{5-5} 
&  ReGVD  & 90.12\%	& 68.36\%	& 43.88\%
\tabularnewline
\cline{2-5} \cline{3-5} \cline{4-5} \cline{5-5} 
&  \multirow{2}{*}{\ourapp~ (Ours)}  & \textbf{0.00\%} & \textbf{99.82\%} & \textbf{99.32\%}
\tabularnewline
%\cline{3-5} \cline{4-5} \cline{5-5} 
 &  & \textcolor{blue}{($\downarrow$ 10.06\%)} & \textcolor{blue}{($\uparrow$ 4.25\%)} & \textcolor{blue}{($\uparrow$ 4.01\%)}\tabularnewline
\hline
%\hline

 \multirow{7}{*}
 &  Standard DNN & 80.08\%	& \underline{90.47\%}	& 18.27\%
 \tabularnewline
%\cline{2-5} \cline{3-5} \cline{4-5} \cline{5-5} 
 &  Outlier Exposure &  86.52\%	& 85.44\%	& 12.84\%
 \tabularnewline
%\cline{2-5} \cline{3-5} \cline{4-5} \cline{5-5} 
{CWE119-20-264}
 &  SSD & 94.34\%	& 79.86\%	& 9.32\%
 \tabularnewline
%\cline{2-5} \cline{3-5} \cline{4-5} \cline{5-5} 
vs. {CWE125}
 &  VulDeePecker & \underline{54.69\%}	& 88.76\%	& \underline{33.41\%}
 \tabularnewline
%\cline{2-5} \cline{3-5} \cline{4-5} \cline{5-5} 
 &  CodeBERT & 90.06\%	& 47.02\%	& 19.17\%
 \tabularnewline
%\cline{2-5} \cline{3-5} \cline{4-5} \cline{5-5} 
 &  ReGVD  & 87.02\%	& 69.85\%	& 8.35\%
 \tabularnewline
\cline{2-5} \cline{3-5} \cline{4-5} \cline{5-5} 
 %&  \ourapp~ (Ours)  & \textbf{0.26\%} & \textbf{99.75\%} & \textbf{92.44\%}
 %\tabularnewline
 & \multirow{2}{*}{\ourapp~ (Ours)} & \textbf{0.00\%} & \textbf{99.93\%} & \textbf{97.06\%}\tabularnewline
%\cline{3-5} \cline{4-5} \cline{5-5} 
 &  & \textcolor{blue}{($\downarrow$ 54.69\%)} & \textcolor{blue}{($\uparrow$ 9.46\%)} & \textcolor{blue}{($\uparrow$ 63.65\%)}\tabularnewline
 \hline
\end{tabular}}
\vspace{-1mm}
\caption{The results of our \ourapp~ method and baselines for the FPR (at TPR 95\%), AUROC, and AUPR measures on the vulnerable source code samples of each out-of-distribution data with the corresponding used in-distribution data. (The best results are in \textbf{bold} while the second highest results are in \underline{underline}. The numbers highlighted in blue color are the improvements of our method \ourapp~ over the second-best values from the baselines.)}\label{tab:my_label_app}
\vspace{-3mm}
\end{table}

\subsection{Discussion of Threats to Validity }\label{sec:discussion}

\paragraph{Construct Validity}
Key construct validity threats are if our assessments of the proposed method and baselines demonstrate their capability for out-of-distribution source code vulnerability detection. In the cyber security domain, by doing out-of-distribution vulnerability detection, we help security analysts and software engineers detect potential unknown vulnerability types coming in order to harden the security computer systems. To evaluate the performance of our method and baselines, we use three main common measures used in out-of-distribution detection including \textbf{FPR} (at TPR 95\%), \textbf{AUROC}, and \textbf{AUPR}.

\paragraph{Internal Validity}
Key internal validity threats are relevant to the choice of hyper-parameter settings (i.e., optimizer, learning rate, number of layers in deep neural networks, etc.). It is worth noting that finding a set of optimal hyperparameter settings of deep neural networks is expensive due to a large number of trainable parameters. To train our method, we only use the common or default values for the hyper-parameters such as using Adam optimizer, the learning rate equals $10^{-3}$, while the scalar temperature $\tau$ used in the cluster-contrastive learning and the temperature $\nu$ for the Gumbel softmax distribution are set in $\{0.5, 1.0\}$. For the number of clusters used in cluster-contrastive learning aiming to improve the data representation learning process, we use it as a hyperparameter. In our paper, we detail the hyperparameter settings (i.e., the value-tuned ranges of the hyperparameters) in the released reproducible source code to support future replication studies.

\paragraph{External Validity}
Key external validity threats include whether our proposed \ourapp~ method will generalize to other source code vulnerability types and whether they will work on other types of vulnerability datasets. We mitigated this problem by conducting our experiments on the top five popular (CWE) vulnerability types as mentioned in \cite{Bigdata2020} including CWE-119 (Improper Restriction of Operations within the Bounds of a Memory Buffer), CWE-20 (Improper Input Validation), CWE-125 (Out-of-bounds Read), CWE-200 (Exposure of Sensitive Information to an Unauthorized Actor), and CWE-264 (Permissions, Privileges, and Access Controls).

\subsection{Additional experiments}\label{sec:additionale}
Here we present some additional experiments of our \ourapp~ method and baselines on other further cases of the in-distribution and out-of-distribution CWE source code data. The experimental results in Table \ref{tab:my_label_app} again show the effectiveness and superiority of our proposed \ourapp~ method compared to the baselines for out-of-distribution CWE identification by a wide margin. Notably, in these additional cases, our method obtains from around (5.56\% to 16.94\%), (0.18\% to 9.37\%), and (1.93\% to 13.82\%) higher performances on the FPR (at TPR 95\%), AUROC, and AUPR measures, respectively, compared to the baselines.
