# Supplementary material for: Deep Learning-Based Out-of-distribution Source Code Data Identification: How Far Have We Gone?
Source: arXiv:2404.05964 source file (2024-04-15)
Supplement: Supplementary file 3 [file supp.tex]

\documentclass[10pt,conference]{IEEEtran}
\IEEEoverridecommandlockouts
\usepackage{cite}
\usepackage{amsmath,amssymb,amsfonts}
\usepackage{algorithmic}
\usepackage{graphicx}
\usepackage{textcomp}
\usepackage{xcolor}
\def\BibTeX{{\rm B\kern-.05em{\sc i\kern-.025em b}\kern-.08em
    T\kern-.1667em\lower.7ex\hbox{E}\kern-.125emX}}

\usepackage{graphicx}
\usepackage{algorithmic}
\usepackage{textcomp}
\usepackage{xcolor}
\usepackage{etoolbox}
\usepackage{multirow}
\usepackage{url}
\usepackage{multirow,booktabs}
\usepackage{subcaption}
\usepackage{wrapfig}
\usepackage{float}
\usepackage{float}
\usepackage{tcolorbox}
\usepackage[flushleft]{threeparttable}
\usepackage{relsize}
\usepackage[inline]{enumitem}
\usepackage{amsmath}

\usepackage{algorithm2e}

\restylefloat{figure}

\begin{document}

\title{LEO: An Innovative Information-theoretic Learning-based
Approach for Identifying Out-of-distribution Source Code Data (Supplementary Material)}

\author{
{\rm Anonymous Author(s)}
}

\maketitle

\input{sections/supp_frameworks}
\input{sections/supp_experiments}

\bibliographystyle{IEEEtran}
\bibliography{reference}

\end{document}
